# Supplementary material for: Hierarchical Representations and Explicit Memory: Learning Effective Navigation Policies on 3D Scene Graphs using Graph Neural Networks
Source: arXiv:2108.01176 source file (2022-05-05)
Supplement: Supplementary file 1 [file classical_methods.tex]

%!TEX root = ../supplemental.tex

\newpage
\highlight{
\section{On the Performance of Model-based Methods}

To motivate the necessity for learned approaches, this section illustrates the challenges faced by a model-based exploration method in our multi-object search problem as described in Section 4.1 of the main paper. 
To this end, we develop a Monte Carlo simulation that mimics our search problem. Where approximations are needed, we simplify in favor of the exploration approach.

We consider an environment of size 1,380\,m$^2$, which is slightly smaller than our smallest evaluation environment, in the form of a 46\,m by 30\,m rectangle. The agent explores the environment via lawnmower patterns using an action space derived from the multi-object search problem.
Specifically, the agent uses two steps to move forward 1\,m, and 11 steps to turn 90 degrees. Thirty targets are randomly placed in the environment, and the agent collects any targets within 2\,m of its current position.
To maximize area coverage, each pass in the agent's trajectory is spaced 4\,m apart.
The agent's initial pose and target locations are randomly set at the start of each episode.

We note that this simulation favors the classical method in several ways.
Unlike our photo-realistic environments, the grid environment contains no narrow passages such as doors or hallways. Thus, the agent does not have to use actions maneuvering in tight spaces. Moreover, the lawnmower pattern is designed to be aligned with the main axes of the room (making it more efficient) and to avoid any collisions (hence implicitly assuming prior knowledge of the environment and robot location).
Moreover, this environment is obstacle free and smaller than all environments we evaluated in 
Table~1 of the main paper.

Monte Carlo results from 10,000 episodes are shown in Table~\ref{tab:exploration}. As expected, the model-based exploration approach does cover more area. However, as the exploration approach cannot guide its trajectory based on environmental cues, the increase in area explored does not translate into more targets found. Note that for the proposed approach we report the same numbers of Table 1 in the main paper (which are obtained in much more complex and larger environments). Despite this disadvantage, the proposed approach still outperforms the model-based exploration baseline by a large margin, in terms of targets found.
% , and despite the fact that the model-based exploration approach is tested on a simpler environment, it still has a large performance gap with respect to the proposed method.

More generally, an effective approach for object search must rely on learning, since the goal is for the navigation policy to learn correlations between the target objects and nodes in the scene graph (\eg which room they are likely to be found in, which objects they are likely to be close to, etc.) --- therefore, an effective policy would spend less time in certain areas and more time in others where objects are likely to be found. A traditional approach (without learning) would only be bound to perform brute-force exploration, which would constitute a suboptimal strategy. 
}
\begin{table}[!h]
    \centering
    \begin{tabular}{llll}
        \toprule
        Method       & Targets Found (\%, $\uparrow$) & Collisions ($\downarrow$)  & Area Explored (m$^2$, $\uparrow$) \\
        \midrule
        Proposed, Complex Env    & \textbf{44.2} (42.7, 45.7)     & 90.0 (84.3, 95.6)          & 59.1 (57.7, 60.5)        \\
        Model-based, Simple Env & 38.5 (38.2, 38.7)             & N/A      &  \textbf{150.6} (150.2, 150.8)                 \\
        \bottomrule
    \end{tabular}
    \caption{Performance of a model-based exploration method in a simplified multi-object search environment. For comparison, we provide results from the proposed method in the full set of evaluation environments. The exploration method does explore more area. However, it collect significantly less targets than the proposed approach as it cannot guide its trajectory based on environmental cues. \label{tab:exploration}}
\end{table}
